# Supplementary material for: Hand-Object Interaction Reasoning
Source: arXiv:2201.04906 source file (2022-01-13)
Supplement: Supplementary file 1 [file supplementary_body.tex]

%\hypersetup{colorlinks = true, linkcolor  = black}

%\startcontents[sections]
%\printcontents[sections]{ }{1}{}
%\clearpage

%\hypersetup{colorlinks = true, linkcolor  = red }
% \section{Positional Encoding}

% Given the detection of hands and objects per frame,  we design a weights-shared 3D ConvNet to learn the positional information from consecutive frames, as Fig.~\ref{fig: spe} shows. Note that while we use local 3D convolution to model motion, we have the position encoding per frame to correspond to the detection bounding box $b$.

% Specifically, the spatial position encoder consists of a 3-layer 3D convolution with the fixed kernel size (5x5), followed by a global average pooling (GAP) across the spatial dimension. Creatively, we adopt binary maps composed of 1 within detections and 0 outside detections. This is able to represent the absolute positions of frame-based objects and hands. We feed consecutive binary maps to the spatial position encoder to learn position features $p$ of hands and objects.
% \begin{figure}[h]
% \centering
% \includegraphics[width=\linewidth]{figs/spe_simplified.pdf}
% \caption{Spatial Position Encoder. Detections, per object, over a sequence are represented by binary maps. A 3-layer 3D ConvNet produces per-frame spatial encoding.}
% \label{fig: spe}
% \end{figure}

% \section{Interaction Unit}

%  We use transformers~\cite{vaswani2017attention} for hand-object reasoning as detailed next. 
%  We model video-based interaction estimation from extracted sequences of left/right hands and interacted objects $\left \{H_{L}, H_{R}, O_{L}, O_{R} \right \}$.

% The proposed Interaction Unit, shown in Fig.~\ref{fig: IU}, consists of a standard encoder and decoder. For the encoder, it aims to reason about the interaction in pairs of $\left \{ H_{L}, H_{R}, O_{L}, O_{R} \right \}$ with a parameters-shared interaction encoder. Hands as actors are typically thought of as queries, with the interacting objects or the other hand being mapped to keys and values. Overall, interaction information is learned by concatenating sub-interactions of all pairings using attention modules and a feedforward neural network. We adopt 4 different MLPs to map visual features to queries, keys and values and feed them to attention blocks. Subsequently, enriched features are summed with the input query to form $E^{'}$ with a residual connection. Therefore, the overall interaction information $E^{''}$ is represented by concatenating all sub-interaction, of both left and right hands.


% Decoders aim to bring together the reasoned hand interactions with the action features. They contain not only hands and objects in the interaction, but also the globally pooled appearance and motion features. For example, the appearance of the sink is very likely to be relevant to recognise the action ``wash fork'', despite it not being the hand or the directly interacting object ``fork''. Specifically, the overall interaction information $E^{''}$ is projected to keys and values as input to decoders which model the interaction between HoI interaction unit output and the globally-pooled action representation. Different from encoders, queries of decodes stem from, and aim to enrich, the action representation. At last, the output of decoders is used for the final classification.

% \begin{figure*}[t]
% \centering
% \includegraphics[width=\linewidth]{figs/interaction_units_simplified.pdf}
% \caption{The Architecture of proposed Interaction Unit (IU). This module includes encoders and decoders. Encoders reason about hand-object interactions by multi-head transformers with hands as query and objects as key and value. Encoders outputs from left and right hands are concatenated and fed to decoders. Decoders model the interaction with action representation.} %Finally, the output is trained for action recognition. }
% \label{fig: IU}
% \end{figure*}


% \section{Implementation Details}

% The hand-object detector~\cite{Shan20} based on Faster-RCNN~\cite{ren2015faster} aims to find links between action performers (hands) and interacting objects by optimising an offset vector per hand~\cite{gkioxari2018detecting}. It not only detects left/right hands and their interacting objects, but also yields directions and distances between hands and contacted objects.

% The hand-object detector~\cite{Shan20} was trained on 100 days dataset that contains both first-person and third-person videos. We use the publicly available trained weights, and detect frame-level hands and objects with the confidence threshold of 0.5.  

% \section{Data Augmentation}

% It is important to note that we changed the random cropping typically used for spatial data augmentation during training. This is because randomly cropping the image in EPIC-KITCHENS-100~\cite{Damen2020RESCALING} results in hands and objects being frequently cropped out of the main frame. As we show in Fig.~\ref{fig: dataAugmentation}, the standard (STD) random cropping from the input image can very likely crop the right hand and plate out. This significantly harms the proposed interaction unit, as the detections are no longer present in the input to the encoder.

% In egocentric footage, hands can be in the bottom half of the image or towards a corner. To avoid this while maintaining the power of augmentation, we first randomly scale (\textbf{S}) frames to ${H}'\times {W}'$, then crop (\textbf{C}) frames to ${H}'\times {H}'$ and finally resize (\textbf{R}) frames to the target resolution $224\times 224$. We refer to this proposed spatial augmentation approach as Scaling-Cropping-Resizing (SCR), which we use in all our experiments on EPIC-KITCHENS-100. 
% We have already compared the two approaches in Table 5 of the main paper showing the importance of this augmentation for our approach (IRN).

% The two data augmentations perform comparably on Something-Else dataset~\cite{materzynska2020something} as the action is typically at the centre of the image.
% We thus use the standard random cropping data augmentation for this dataset.

% \begin{figure*}[t]
% \centering
% \includegraphics[width=0.95\textwidth]{figs/dataAugmentation.pdf}
% \caption{Visualisation of STD and SCR for data augmentation. Sample image from EPIC-KITCHENS-100 for the action ``take plate''.}
% \label{fig: dataAugmentation}
% \end{figure*}





% \section{Ablation Study}

% We present three additional ablations in this section.

% \begin{table}[t]
% % \hspace{0.15cm}
% \begin{minipage}[t]{0.25\linewidth}
% \footnotesize
% \begin{center}
% \begin{tabular}{ll}
% \hline
% %   & \multicolumn{3}{l}{Top-1 Accuracy (\%)} \\ \cline{2-4}
%  SPE          & Top-1   \\ \hline
%  none            &43.39   \\
%  concat        &42.71  \\
%  sum         &\textbf{44.52}  \\ \hline
% \end{tabular}
% \end{center}
% \caption{Ablation study for Spatial Position Encoding. }
% \label{tbl: inter sep}
% \end{minipage}
% \hspace{0.05\linewidth}
% \begin{minipage}[t]{0.25\linewidth}
% \footnotesize
% \begin{center}
% \begin{tabular}{ll}
% \hline
% %   & \multicolumn{3}{l}{Top-1 Accuracy (\%)} \\ \cline{2-4}
%  Act.Rep.       &Top-1  \\ \hline
%  none        &31.98  \\
%  concat   &43.73 \\
%  decoder  &\textbf{44.52}  \\ \hline
% \end{tabular}
% \end{center}
% \caption{Ablation study for Action Representation.}
% \label{tbl: context}
% \end{minipage}
% \hspace{0.05\linewidth}
% \begin{minipage}[t]{0.25\linewidth}
% \footnotesize
% \begin{center}
% \begin{tabular}{ll}
% \hline
% %   & \multicolumn{3}{l}{Top-1 Accuracy (\%)} \\ \cline{2-4}
% Det.Rep       &Top-1  \\ \hline
%  MLP   &43.95 \\
%  CNN  &\textbf{44.52}  \\ \hline
% \end{tabular}
% \end{center}
% \caption{Ablation study for Detection Representation.}
% \label{tbl: vfe}
% \end{minipage}
% \end{table}

% \noindent \textbf{Spatial Positional Encoding.} We adopt two ways to fuse positional information with visual features of hands or objects. As we expected in Tab.~\ref{tbl: inter sep}, spatial position encoding $SPE$ improves the performance. Compared to the network without $SPE$ ($none$ in Tab.~\ref{tbl: inter sep}) or concatenations of $SPE$. This is due to the sparsity of positional features. Concatenating lots of zeros to the visual features may introduce noise. Our proposed approach to $sum$ the positional encoding yields the best action performance.



% \noindent \textbf{Action Representation.} In this ablation study, we evaluate the importance of globally pooled action representation. First, we remove the decoders
% % that aims to learn the interaction between hand-object interaction and the action representation, which contains contextual information from the whole frame. We 
% and train the network with only interaction features, i.e. $none$.
% This would be the output of the encoer solely.
% Tab.~\ref{tbl: context} shows that results drop significantly if the network does not use the globally-pooled action representation. We also concatenate the hand-object interactions with the action representation, in a late-fusion fashion.
% % , which is commonly used in other works~\cite{sun2018actor, pan2020actor}. 
% What stands out in the Tab.~\ref{tbl: context} is that the Top-1 action result of the decoder surpasses concatenation. %Particularly, the noun accuracy of our decoders outperform concatenation's by 1.81\%. Hence, our decoders have a better ability in modeling interactions.

% \noindent \textbf{Detection Representation.} 
% In all other experiments, we have used RoI pooling to get feature representations of our hands' and objects' detections. 
% Instead, inspired by popular MLPs~\cite{tolstikhin2021mlp}, we also explore using MLP projection directly from image patches. We crop the input image given bounding boxes $b$ and resize to a fixed size by bilinear interpolation. The fixed size patches are flatten, and projected using an MLP. 
% Hence, representations of any detections can be learned by a parameter-shared MLP. Notably, these features only contain the spatial information, without any motion cues as they are projected per image. We compare performances of MLPs and pooled 3D-CNN as the features extractors. Tab.~\ref{tbl: vfe} shows that the accuracy of 3D-CNN pooling is superior to MLP projection, indicating that temporal features are significant for video-based hand-to-object interactions.
